# Supplementary material for: Performance Aware Convolutional Neural Network Channel Pruning for Embedded GPUs
Source: arXiv:2002.08697 source file (2020-02-20)
Supplement: Supplementary file 1 [file appendix.tex]

\clearpage

\section*{Appendix - All layer charts}\label{sec:appendix}

\subsection{Arm CompLib GEMM on HiKey}

\begin{figure}
    \centering
    \includegraphics[width=\columnwidth]{images/layers/hikey/g_l0.pdf}
    \caption{Layer 0 with GEMM on HiKey 970}
\end{figure}

\begin{figure}
    \centering
    \includegraphics[width=\columnwidth]{images/layers/hikey/g_l1.pdf}
    \caption{Layer 1 with GEMM on HiKey 970}
\end{figure}

\begin{figure}
    \centering
    \includegraphics[width=\columnwidth]{images/layers/hikey/g_l2.pdf}
    \caption{Layer 2 with GEMM on HiKey 970}
\end{figure}

\begin{figure}
    \centering
    \includegraphics[width=\columnwidth]{images/layers/hikey/g_l3.pdf}
    \caption{Layer 3 with GEMM on HiKey 970}
\end{figure}

\begin{figure}
    \centering
    \includegraphics[width=\columnwidth]{images/layers/hikey/g_l5.pdf}
    \caption{Layer 5 with GEMM on HiKey 970}
\end{figure}

\begin{figure}
    \centering
    \includegraphics[width=\columnwidth]{images/layers/hikey/g_l11.pdf}
    \caption{Layer 11 with GEMM on HiKey 970}
\end{figure}

\begin{figure}
    \centering
    \includegraphics[width=\columnwidth]{images/layers/hikey/g_l12.pdf}
    \caption{Layer 12 with GEMM on HiKey 970}
\end{figure}

\begin{figure}
    \centering
    \includegraphics[width=\columnwidth]{images/layers/hikey/g_l13.pdf}
    \caption{Layer 13 with GEMM on HiKey 970}
\end{figure}

\begin{figure}
    \centering
    \includegraphics[width=\columnwidth]{images/layers/hikey/g_l14.pdf}
    \caption{Layer 14 with GEMM on HiKey 970}
\end{figure}

\begin{figure}
    \centering
    \includegraphics[width=\columnwidth]{images/layers/hikey/g_l15.pdf}
    \caption{Layer 15 with GEMM on HiKey 970}
\end{figure}

\begin{figure}
    \centering
    \includegraphics[width=\columnwidth]{images/layers/hikey/g_l16.pdf}
    \caption{Layer 16 with GEMM on HiKey 970}
\end{figure}

\begin{figure}
    \centering
    \includegraphics[width=\columnwidth]{images/layers/hikey/g_l24.pdf}
    \caption{Layer 24 with GEMM on HiKey 970}
\end{figure}

\begin{figure}
    \centering
    \includegraphics[width=\columnwidth]{images/layers/hikey/g_l25.pdf}
    \caption{Layer 25 with GEMM on HiKey 970}
\end{figure}

\begin{figure}
    \centering
    \includegraphics[width=\columnwidth]{images/layers/hikey/g_l26.pdf}
    \caption{Layer 26 with GEMM on HiKey 970}
\end{figure}

\begin{figure}
    \centering
    \includegraphics[width=\columnwidth]{images/layers/hikey/g_l27.pdf}
    \caption{Layer 27 with GEMM on HiKey 970}
\end{figure}

\begin{figure}
    \centering
    \includegraphics[width=\columnwidth]{images/layers/hikey/g_l28.pdf}
    \caption{Layer 28 with GEMM on HiKey 970}
\end{figure}

\begin{figure}
    \centering
    \includegraphics[width=\columnwidth]{images/layers/hikey/g_l29.pdf}
    \caption{Layer 29 with GEMM on HiKey 970}
\end{figure}

\begin{figure}
    \centering
    \includegraphics[width=\columnwidth]{images/layers/hikey/g_l43.pdf}
    \caption{Layer 43 with GEMM on HiKey 970}
\end{figure}

\begin{figure}
    \centering
    \includegraphics[width=\columnwidth]{images/layers/hikey/g_l44.pdf}
    \caption{Layer 44 with GEMM on HiKey 970}
\end{figure}

\begin{figure}
    \centering
    \includegraphics[width=\columnwidth]{images/layers/hikey/g_l45.pdf}
    \caption{Layer 45 with GEMM on HiKey 970}
\end{figure}

\begin{figure}
    \centering
    \includegraphics[width=\columnwidth]{images/layers/hikey/g_l46.pdf}
    \caption{Layer 46 with GEMM on HiKey 970}
\end{figure}

\begin{figure}
    \centering
    \includegraphics[width=\columnwidth]{images/layers/hikey/g_l47.pdf}
    \caption{Layer 47 with GEMM on HiKey 970}
\end{figure}

\begin{figure}
    \centering
    \includegraphics[width=\columnwidth]{images/layers/hikey/g_l48.pdf}
    \caption{Layer 48 with GEMM on HiKey 970}
\end{figure}

%%%%%%%%%%%%%%%%%%%

\subsection{VGG on HiKey with GEMM implementation of Arm Compute Library}

\begin{figure}
    \centering
    \includegraphics[width=\columnwidth]{images/layers/hikey_vgg/g_l0.pdf}
    \caption{Layer 0 of VGG with Arm Compute Library GEMM on HiKey 970}
\end{figure}

\begin{figure}
    \centering
    \includegraphics[width=\columnwidth]{images/layers/hikey_vgg/g_l2.pdf}
    \caption{Layer 2 of VGG with Arm Compute Library GEMM on HiKey 970}
\end{figure}

\begin{figure}
    \centering
    \includegraphics[width=\columnwidth]{images/layers/hikey_vgg/g_l5.pdf}
    \caption{Layer 5 of VGG with Arm Compute Library GEMM on HiKey 970}
\end{figure}

\begin{figure}
    \centering
    \includegraphics[width=\columnwidth]{images/layers/hikey_vgg/g_l7.pdf}
    \caption{Layer 7 of VGG with Arm Compute Library GEMM on HiKey 970}
\end{figure}

\begin{figure}
    \centering
    \includegraphics[width=\columnwidth]{images/layers/hikey_vgg/g_l10.pdf}
    \caption{Layer 10 of VGG with Arm Compute Library GEMM on HiKey 970}
\end{figure}

\begin{figure}
    \centering
    \includegraphics[width=\columnwidth]{images/layers/hikey_vgg/g_l12.pdf}
    \caption{Layer 12 of VGG with Arm Compute Library GEMM on HiKey 970}
\end{figure}

\begin{figure}
    \centering
    \includegraphics[width=\columnwidth]{images/layers/hikey_vgg/g_l17.pdf}
    \caption{Layer 17 of VGG with Arm Compute Library GEMM on HiKey 970}
\end{figure}

\begin{figure}
    \centering
    \includegraphics[width=\columnwidth]{images/layers/hikey_vgg/g_l19.pdf}
    \caption{Layer 19 of VGG with Arm Compute Library GEMM on HiKey 970}
\end{figure}

\begin{figure}
    \centering
    \includegraphics[width=\columnwidth]{images/layers/hikey_vgg/g_l24.pdf}
    \caption{Layer 24 of VGG with Arm Compute Library GEMM on HiKey 970}
\end{figure}

%%%%%%%%%%%%%%%%%%%%%%%%%%%%%%%%%%%%%%%%

\subsection{CuDNN on TX2}

\begin{figure}
    \centering
    \includegraphics[width=\columnwidth]{images/layers/tx2_resnet/g_l0.pdf}
    \caption{Layer 0 of ResNet with CuDNN on Jetson TX2.}
\end{figure}

\begin{figure}
    \centering
    \includegraphics[width=\columnwidth]{images/layers/tx2_resnet/g_l1.pdf}
    \caption{Layer 1 of ResNet with CuDNN on Jetson TX2.}
\end{figure}

\begin{figure}
    \centering
    \includegraphics[width=\columnwidth]{images/layers/tx2_resnet/g_l2.pdf}
    \caption{Layer 2 of ResNet with CuDNN on Jetson TX2.}
\end{figure}

\begin{figure}
    \centering
    \includegraphics[width=\columnwidth]{images/layers/tx2_resnet/g_l3.pdf}
    \caption{Layer 3 of ResNet with CuDNN on Jetson TX2.}
\end{figure}

\begin{figure}
    \centering
    \includegraphics[width=\columnwidth]{images/layers/tx2_resnet/g_l5.pdf}
    \caption{Layer 5 of ResNet with CuDNN on Jetson TX2.}
\end{figure}

\begin{figure}
    \centering
    \includegraphics[width=\columnwidth]{images/layers/tx2_resnet/g_l11.pdf}
    \caption{Layer 11 of ResNet with CuDNN on Jetson TX2.}
\end{figure}

\begin{figure}
    \centering
    \includegraphics[width=\columnwidth]{images/layers/tx2_resnet/g_l12.pdf}
    \caption{Layer 12 of ResNet with CuDNN on Jetson TX2.}
\end{figure}

\begin{figure}
    \centering
    \includegraphics[width=\columnwidth]{images/layers/tx2_resnet/g_l13.pdf}
    \caption{Layer 13 of ResNet with CuDNN on Jetson TX2.}
\end{figure}

\begin{figure}
    \centering
    \includegraphics[width=\columnwidth]{images/layers/tx2_resnet/g_l14.pdf}
    \caption{Layer 14 of ResNet with CuDNN on Jetson TX2.}
\end{figure}

\begin{figure}
    \centering
    \includegraphics[width=\columnwidth]{images/layers/tx2_resnet/g_l15.pdf}
    \caption{Layer 15 of ResNet with CuDNN on Jetson TX2.}
\end{figure}

\begin{figure}
    \centering
    \includegraphics[width=\columnwidth]{images/layers/tx2_resnet/g_l16.pdf}
    \caption{Layer 16 of ResNet with CuDNN on Jetson TX2.}
\end{figure}

\begin{figure}
    \centering
    \includegraphics[width=\columnwidth]{images/layers/tx2_resnet/g_l24.pdf}
    \caption{Layer 24 of ResNet with CuDNN on Jetson TX2.}
\end{figure}

\begin{figure}
    \centering
    \includegraphics[width=\columnwidth]{images/layers/tx2_resnet/g_l25.pdf}
    \caption{Layer 25 of ResNet with CuDNN on Jetson TX2.}
\end{figure}

\begin{figure}
    \centering
    \includegraphics[width=\columnwidth]{images/layers/tx2_resnet/g_l26.pdf}
    \caption{Layer 26 of ResNet with CuDNN on Jetson TX2.}
\end{figure}

\begin{figure}
    \centering
    \includegraphics[width=\columnwidth]{images/layers/tx2_resnet/g_l27.pdf}
    \caption{Layer 27 of ResNet with CuDNN on Jetson TX2.}
\end{figure}

%%%%%%%%%%%%%%%%%%%%

\subsection{CuDNN on Nano}

\begin{figure}
    \centering
    \includegraphics[width=\columnwidth]{images/layers/nano_resnet/g_l0.pdf}
    \caption{Layer 0 of ResNet with CuDNN on Jetson Nano.}
\end{figure}

\begin{figure}
    \centering
    \includegraphics[width=\columnwidth]{images/layers/nano_resnet/g_l1.pdf}
    \caption{Layer 1 of ResNet with CuDNN on Jetson Nano.}
\end{figure}

\newpage
%%%%%%%%%%%%%%%%%%%%%%

\subsection{Arm CompLib Direct Conv. on HiKey}

\begin{figure}
    \centering
    \includegraphics[width=\columnwidth]{images/layers/hikey/d_l0.pdf}
    \caption{Layer 0 with Direct on HiKey 970}
\end{figure}

\begin{figure}
    \centering
    \includegraphics[width=\columnwidth]{images/layers/hikey/d_l1.pdf}
    \caption{Layer 1 with Direct on HiKey 970}
\end{figure}

\begin{figure}
    \centering
    \includegraphics[width=\columnwidth]{images/layers/hikey/d_l2.pdf}
    \caption{Layer 2 with Direct on HiKey 970}
\end{figure}

\begin{figure}
    \centering
    \includegraphics[width=\columnwidth]{images/layers/hikey/d_l3.pdf}
    \caption{Layer 3 with Direct on HiKey 970}
\end{figure}

\begin{figure}
    \centering
    \includegraphics[width=\columnwidth]{images/layers/hikey/d_l5.pdf}
    \caption{Layer 5 with Direct on HiKey 970}
\end{figure}

\begin{figure}
    \centering
    \includegraphics[width=\columnwidth]{images/layers/hikey/d_l11.pdf}
    \caption{Layer 11 with Direct on HiKey 970}
\end{figure}

\begin{figure}
    \centering
    \includegraphics[width=\columnwidth]{images/layers/hikey/d_l12.pdf}
    \caption{Layer 12 with Direct on HiKey 970}
\end{figure}

\begin{figure}
    \centering
    \includegraphics[width=\columnwidth]{images/layers/hikey/d_l13.pdf}
    \caption{Layer 13 with Direct on HiKey 970}
\end{figure}

\begin{figure}
    \centering
    \includegraphics[width=\columnwidth]{images/layers/hikey/d_l14.pdf}
    \caption{Layer 14 with Direct on HiKey 970}
\end{figure}

\begin{figure}
    \centering
    \includegraphics[width=\columnwidth]{images/layers/hikey/d_l15.pdf}
    \caption{Layer 15 with Direct on HiKey 970}
\end{figure}

\begin{figure}
    \centering
    \includegraphics[width=\columnwidth]{images/layers/hikey/d_l16.pdf}
    \caption{Layer 16 with Direct on HiKey 970}
\end{figure}

\begin{figure}
    \centering
    \includegraphics[width=\columnwidth]{images/layers/hikey/d_l24.pdf}
    \caption{Layer 24 with Direct on HiKey 970}
\end{figure}

\begin{figure}
    \centering
    \includegraphics[width=\columnwidth]{images/layers/hikey/d_l25.pdf}
    \caption{Layer 25 with Direct on HiKey 970}
\end{figure}

\begin{figure}
    \centering
    \includegraphics[width=\columnwidth]{images/layers/hikey/d_l26.pdf}
    \caption{Layer 26 with Direct on HiKey 970}
\end{figure}

\begin{figure}
    \centering
    \includegraphics[width=\columnwidth]{images/layers/hikey/d_l27.pdf}
    \caption{Layer 27 with Direct on HiKey 970}
\end{figure}

\begin{figure}
    \centering
    \includegraphics[width=\columnwidth]{images/layers/hikey/d_l28.pdf}
    \caption{Layer 28 with Direct on HiKey 970}
\end{figure}

\begin{figure}
    \centering
    \includegraphics[width=\columnwidth]{images/layers/hikey/d_l29.pdf}
    \caption{Layer 29 with Direct on HiKey 970}
\end{figure}

\begin{figure}
    \centering
    \includegraphics[width=\columnwidth]{images/layers/hikey/d_l43.pdf}
    \caption{Layer 43 with Direct on HiKey 970}
\end{figure}

\begin{figure}
    \centering
    \includegraphics[width=\columnwidth]{images/layers/hikey/d_l44.pdf}
    \caption{Layer 44 with Direct on HiKey 970}
\end{figure}

\begin{figure}
    \centering
    \includegraphics[width=\columnwidth]{images/layers/hikey/d_l45.pdf}
    \caption{Layer 45 with Direct on HiKey 970}
\end{figure}

\begin{figure}
    \centering
    \includegraphics[width=\columnwidth]{images/layers/hikey/d_l46.pdf}
    \caption{Layer 46 with Direct on HiKey 970}
\end{figure}

\begin{figure}
    \centering
    \includegraphics[width=\columnwidth]{images/layers/hikey/d_l47.pdf}
    \caption{Layer 47 with Direct on HiKey 970}
\end{figure}

\begin{figure}
    \centering
    \includegraphics[width=\columnwidth]{images/layers/hikey/d_l48.pdf}
    \caption{Layer 48 with Direct on HiKey 970}
\end{figure}

\newpage
%%%%%%%%%%%%%%%%%%%%%%

\subsection{TVM on HiKey}

\begin{figure}
    \centering
    \includegraphics[width=\columnwidth]{images/layers/hikey/tvm_l0.pdf}
    \caption{Layer 0 with TVM on HiKey 970}
\end{figure}

\begin{figure}
    \centering
    \includegraphics[width=\columnwidth]{images/layers/hikey/tvm_l1.pdf}
    \caption{Layer 1 with TVM on HiKey 970}
\end{figure}

\begin{figure}
    \centering
    \includegraphics[width=\columnwidth]{images/layers/hikey/tvm_l2.pdf}
    \caption{Layer 2 with TVM on HiKey 970}
\end{figure}

\begin{figure}
    \centering
    \includegraphics[width=\columnwidth]{images/layers/hikey/tvm_l3.pdf}
    \caption{Layer 3 with TVM on HiKey 970}
\end{figure}

\begin{figure}
    \centering
    \includegraphics[width=\columnwidth]{images/layers/hikey/tvm_l5.pdf}
    \caption{Layer 5 with TVM on HiKey 970}
\end{figure}

\begin{figure}
    \centering
    \includegraphics[width=\columnwidth]{images/layers/hikey/tvm_l11.pdf}
    \caption{Layer 11 with TVM on HiKey 970}
\end{figure}

\begin{figure}
    \centering
    \includegraphics[width=\columnwidth]{images/layers/hikey/tvm_l12.pdf}
    \caption{Layer 12 with TVM on HiKey 970}
\end{figure}

\begin{figure}
    \centering
    \includegraphics[width=\columnwidth]{images/layers/hikey/tvm_l13.pdf}
    \caption{Layer 13 with TVM on HiKey 970}
\end{figure}

\begin{figure}
    \centering
    \includegraphics[width=\columnwidth]{images/layers/hikey/tvm_l14.pdf}
    \caption{Layer 14 with TVM on HiKey 970}
\end{figure}

\begin{figure}
    \centering
    \includegraphics[width=\columnwidth]{images/layers/hikey/tvm_l15.pdf}
    \caption{Layer 15 with TVM on HiKey 970}
\end{figure}

\begin{figure}
    \centering
    \includegraphics[width=\columnwidth]{images/layers/hikey/tvm_l16.pdf}
    \caption{Layer 16 with TVM on HiKey 970}
\end{figure}

\begin{figure}
    \centering
    \includegraphics[width=\columnwidth]{images/layers/hikey/tvm_l24.pdf}
    \caption{Layer 24 with TVM on HiKey 970}
\end{figure}

\begin{figure}
    \centering
    \includegraphics[width=\columnwidth]{images/layers/hikey/tvm_l25.pdf}
    \caption{Layer 25 with TVM on HiKey 970}
\end{figure}

\begin{figure}
    \centering
    \includegraphics[width=\columnwidth]{images/layers/hikey/tvm_l26.pdf}
    \caption{Layer 26 with TVM on HiKey 970}
\end{figure}

\begin{figure}
    \centering
    \includegraphics[width=\columnwidth]{images/layers/hikey/tvm_l27.pdf}
    \caption{Layer 27 with TVM on HiKey 970}
\end{figure}

\begin{figure}
    \centering
    \includegraphics[width=\columnwidth]{images/layers/hikey/tvm_l28.pdf}
    \caption{Layer 28 with TVM on HiKey 970}
\end{figure}

\begin{figure}
    \centering
    \includegraphics[width=\columnwidth]{images/layers/hikey/tvm_l29.pdf}
    \caption{Layer 29 with TVM on HiKey 970}
\end{figure}

\begin{figure}
    \centering
    \includegraphics[width=\columnwidth]{images/layers/hikey/tvm_l43.pdf}
    \caption{Layer 43 with TVM on HiKey 970}
\end{figure}

\begin{figure}
    \centering
    \includegraphics[width=\columnwidth]{images/layers/hikey/tvm_l44.pdf}
    \caption{Layer 44 with TVM on HiKey 970}
\end{figure}

\begin{figure}
    \centering
    \includegraphics[width=\columnwidth]{images/layers/hikey/tvm_l45.pdf}
    \caption{Layer 45 with TVM on HiKey 970}
\end{figure}

\begin{figure}
    \centering
    \includegraphics[width=\columnwidth]{images/layers/hikey/tvm_l46.pdf}
    \caption{Layer 46 with TVM on HiKey 970}
\end{figure}

\begin{figure}
    \centering
    \includegraphics[width=\columnwidth]{images/layers/hikey/tvm_l47.pdf}
    \caption{Layer 47 with TVM on HiKey 970}
\end{figure}
